# Supplementary material for: PoseTriplet: Co-evolving 3D Human Pose Estimation, Imitation, and Hallucination under Self-supervision
Source: arXiv:2203.15625 source file (2022-03-29)
Supplement: Supplementary file 1 [file appendix.tex]

In this document, we provide supplementary materials
that cannot fit the manuscript 
due to page limit. Specifically,
we provide details on implementation,
more experimental results, and 
details on the pose estimator, imitator, and hallucinator, 
and discussion on negative social impact.

\section{Implementation details}

\noindent 
We implement \nameofmethod{} using Pytorch~\cite{paszke2017automatic}, and train \nameofmethod{} on a machine with a Intel Xeon Gold 6278C CPU and a Tesla T4 GPU. The whole training process takes 3 rounds for 7 days.
The implementation details for each module are described as follows.

\noindent \textbf{Estimator.}
In pose estimator $\mathcal{P}$, the network parameter is optimized by the Adam~\cite{kingma2014adam} optimizer with a learning rate of $0.0003$ and the linearly decay strategy.

\noindent \textbf{Imitator.}
In pose imitator $\mathcal{I}$, the policy runs at a frequency of 30Hz. 
Proximal policy optimization (PPO)~\cite{schulman2017proximal} is used to update the parameter of policy network with a learning rate of $0.00005$ and Adam optimizer.
We use Mujoco~\cite{todorov2012mujoco}~(open-source) as the physics simulator.
% , with total iteration number 3000 for each round.

\noindent \textbf{Hallucinator.}
Pose hallucinator $\mathcal{H}$ contains a generator and discriminator. The generator is trained with learning rate of $0.0001$, and the discriminator is trained with learning rate of $0.00001$.
Both generator and discriminator are optimized with Adam optimizer.

\section{Experiments}

\subsection{More qualitative results}
We provide a video file ``4806-supp.mp4'' which includes  Fig.~\textcolor{red}{3-8} in video format for better visualization quality. 
In this video, 
we firstly illustrate how \nameofmethod{} progressively generates, refines the 3D motion data from round 1 to 3.
Then we provide more self-generated examples from both imitator and hallucinator.
After that we provide pose estimation results similar to Fig.~\textcolor{red}{3-6} in source dataset (\ie, H36M), cross dataset (\ie, 3DHP and 3DPW), and videos from in-the-wild scenario (\ie, self-collected from TikTok~\cite{jafarian2021tiktok} and Youtube).
Finally  we provide more results for imitator in Fig.~\textcolor{red}{7} and hallucinator in Fig.~\textcolor{red}{8}.
Note that all of these results are achieved
with only monocular 2D pose or video, 
\emph{without} any 3D data or multi-view setting.
This demonstrates 
the robustness of
our \nameofmethod{}
to challenging scenarios, again even 
without the necessity of 
acquiring 3D data.

% \xwc{checked up to here.}

\subsection{More ablation studies}

% \subsubsection{Ablation on the hallucinator}
% 这一段和另外一个{Ablations on co-evolving components} 内容重叠, 两个只留一个.
% %We compared our method with and without hallucinator.
% We report the MPJPE on three public datasets~(\ie, H36M, 3DHP, 3DPW) 
% with and without hallucinator.
% As shown in Table.~\ref{tab:aba-div}, 
% benefiting from the diverse and plausible hallucination data, 
% the hallucinator improves the pose estimator performances 
% on both source and in-the-wild dataset.

% \begin{table}[h]
% 	\small
% 	\centering
% 	\setlength{\tabcolsep}{1mm}
% % 	\vspace{-3mm}
% 	\begin{tabular}{l|c|c|c|c}
% 		\specialrule{1pt}{1pt}{1pt}
% 		Mode & hallucinator  & H36M & 3DHP & 3DPW  \\
% 		\hline
% 		Self &  & 75.6 & 82.7  & 124.2   \\
% 		Self & \checkmark & 68.2 & 79.5  & 115.0   \\
% 		\specialrule{1pt}{1pt}{2pt}	
% 	\end{tabular}
	
% 	\caption{\textbf{Results on ablation with and without hallucinator} in terms of MPJPE.}
% 	\label{tab:aba-div}

% \end{table} 

\subsubsection{Ablation on extra round of co-evolving}
{We here explore more rounds of co-evolving. As shown in Fig.~\ref{fig:aba-round}, the performance saturated after round 4, implying the framework has reached the ceiling of its capacity. }

\begin{figure}[!t]
\centering
\includegraphics[width=0.95\linewidth]{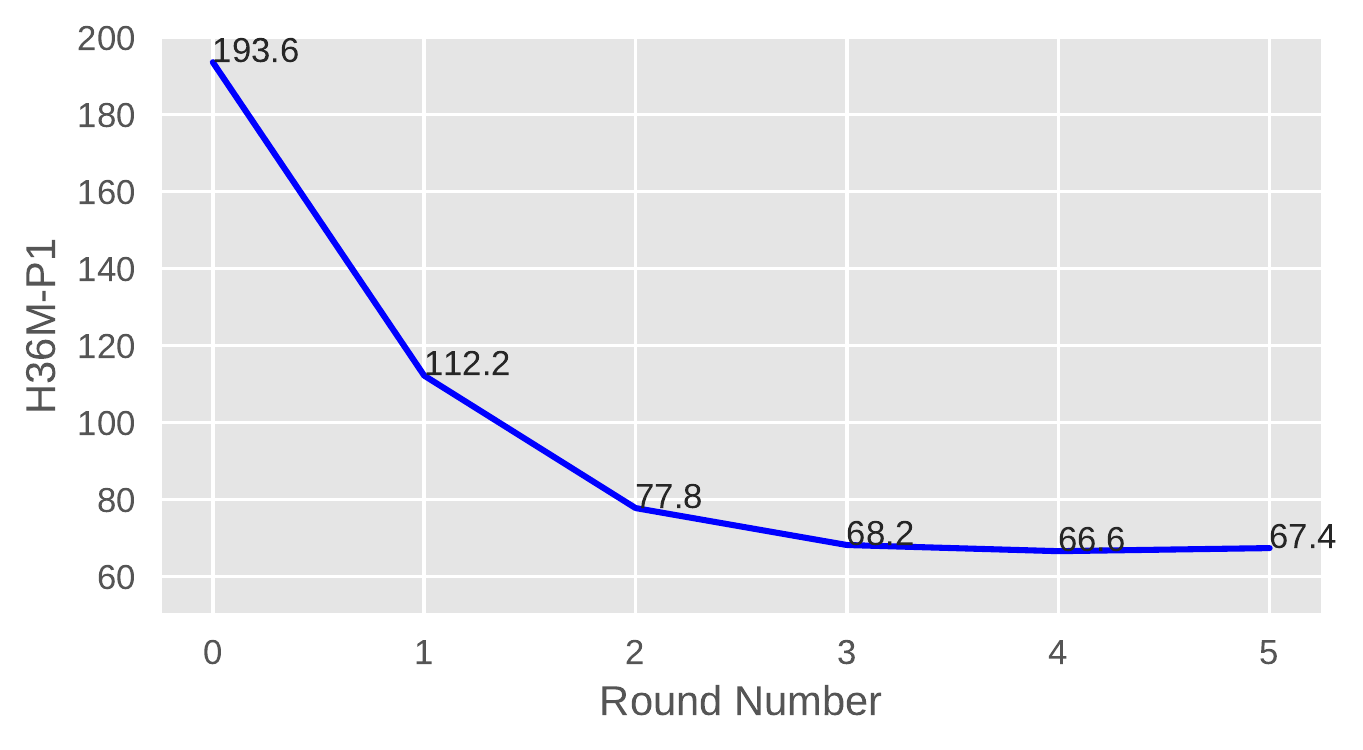}
\caption{Results w.r.t. P1 in H36M with GT2D about Round Number.}
\label{fig:aba-round}
\end{figure}

% \begin{table}[h]
% 	\small
% 	\centering
% 	\setlength{\tabcolsep}{1mm}
% % 	\vspace{-3mm}
%     \begin{tabular}{l|c|c|c|c|c|c}
% % 		\specialrule{1pt}{1pt}{1pt}
% 		Round Num. & 0 & 1 & 2 & 3 & 4 & 5  \\
% 		\hline
% 		Ours (PCA) & 193.6 & 112.2 & 77.8 & 68.2 & 66.6 & 67.4 \\
% 		Ours (Oracle) & 194.8 & 111.3 & 76.6 & 66.5 & 65.2 & 66.5 \\
% % 		\specialrule{1pt}{1pt}{2pt}	
% 	\end{tabular}
% % 	\vspace{-3mm}
% 	\caption{Results w.r.t. P1 in H36M with GT2D. PCA and Oracle denote the approximated and GT ground plane used in the training loop for keeping the simulated character standing up-right. }
% 	\label{tab:aba-round}

% \end{table} 

\subsubsection{Ablations on co-evolving components} 
{To verify the effectiveness of each component in this \nameofmethod{} framework, we here ablate the performance of the estimator without using imitator or hallucinator or both. 
The result in H36M with GT2D w.r.t. P2 are E: 115.8, E+H: 80.3, E+I: 57.6, E+I+H: 45.1, with E, I, H being estimator, imitator, hallucinator. 
This demonstrates that involving either I or H into the framework produces better results. Combining them jointly improves the performance by a large margin.
}

\subsubsection{Ablation on camera pose generator.}
{
We use two camera projection methods (random- and GAN-based camera projection).
% We set the random camera with elevation (0 to 30 degree) and depth (3 to 6 meter) to cover the plausible viewpoint. 
% while increase this range caused unstable training due to the unusual viewpoint, 
% We deployed a GAN based camera to explore plausible viewpoint in a larger range (-90 to 90 degree) and depth ($<$30 meter).
As shown in Table~\ref{tab:aba-cam} (Random and GAN denote random and GAN based camera projection), either method achieves a good performance, combining them together further improves the results.
%due to more diverse viewpoint augmentation.
}

\begin{table}[h]
	\small
	\centering
	\setlength{\tabcolsep}{3mm}
    \begin{tabular}{l|c|c}
    % 		\specialrule{1pt}{1pt}{1pt}
    Camera projection & GT & Det\\
    \hline
    Random  & 74.1 & 80.5\\
    %  Videopose(27) + GT3D  & 39.9 (40.6) & 69.4 & 101.8 \\
    GAN  & 75.6 & 82.9\\
    Random+GAN & 68.2 & 78.0\\
    % 		\specialrule{1pt}{1pt}{2pt}	
    \end{tabular}
    % \vspace{-3mm}
    \caption{Ablation on camera projection in H36M (P1).}
    % \vspace{-6mm}
    \label{tab:aba-cam}

\end{table}

\subsubsection{Ablation on the physics-based pose metrics.}
{
While results of the estimator suffer from physically implausible artifacts (\eg, foot skating (FS) and ground penetration (GP)), 
the imitator helps resolve these issues as shown in  Table~\ref{tab:phymetrics}.
This ensures the plausibility of training set to sever as training data for pose estimator during co-evolving.
}

\begin{table}[h]
	\small
	\centering
	\setlength{\tabcolsep}{3mm}
% 	\vspace{-3mm}
    \begin{tabular}{l|cc|cc}
    % \specialrule{1pt}{1pt}{1pt}
    Method &  \multicolumn{2}{c|}{Train} & \multicolumn{2}{c}{Test}  \\
      &  FS & GP &  FS & GP  \\
    \hline
    w/o I & 7.1  & 2.4 & 6.5 & 3.8 \\	
    w/ I &  0.7 & 0.9 & 0.9 & 1.5 \\	
    % \specialrule{1pt}{1pt}{2pt}	
    \end{tabular}
    % \vspace{-3mm}
    \caption{Results on H36M train and test sets w.r.t. physics-based metrics.}
    \label{tab:phymetrics}

\end{table}

\section{Methodology}

\nameofmethod{} is the first attempt to train three difference pose related tasks jointly in an self-supervised manner. 
Therefore we choose those modules based on solid and simple strategy, and they are flexible to replace by other modules with similar function.
In the following section, we will elaborate the more details for the pose estimator, imitator, and hallucinator.

% \section{More details about pose imitator}

%%%%%%%%%%%%%%% detail of pose estimator - start %%%%%%%%%%%%%
\begin{figure}[h]
\centering
\includegraphics[width=0.95\linewidth]{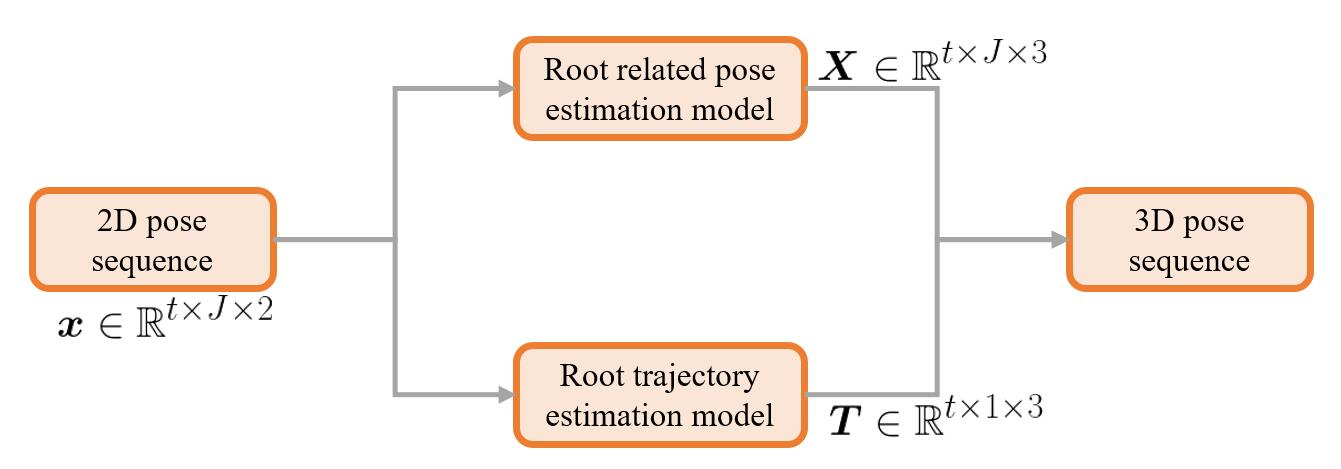}
\caption{\textbf{Pose estimator overview.}}
\label{fig:estimator}
\end{figure}

\subsection{Pose estimator}
% \vspace{-1mm}
% The pose estimator estimates the 3D pose sequence $\boldsymbol{X}_{1:T}$ from the input sequence $\boldsymbol{x}_{1:T}$. 
% % We find the common root-relative motion is ineffective for pose imitator learning as it cannot differentiate different movement with similar root-related motion ~\cite{}.
% Specifically, we adopt a similar estimator architecture as VideoPose~\cite{pavllo2019videopose3d}, which predicts both root trajectory and root-relative joint locations. The trajectory can be used as additional movement signal to pose imitator.
% Meanwhile, the noise in root movement can be corrected by the pose imitator and in turn help the pose estimator.
{
For the pose estimator, we adopt the 1D convolution based VideoPose~\cite{pavllo2019videopose3d}.
Fig.~\ref{fig:estimator} illustrates the architecture of pose estimator. 
It contains two branches: root relative pose estimation and root trajectory estimation.
Given the input 2D pose sequence $\boldsymbol{x}_{1:T}$, these two branches can predict the root relative pose and root trajectory, which are then combined as the output 3D pose sequence $\boldsymbol{X}_{1:T}$\textbf{}, and served as reference motion for imitator.
}
% We use Mean Square Error (MSE) loss for the root-related pose estimation and Weighted L1 loss for the trajectory estimation following~\cite{pavllo2019videopose3d}.

% \noindent \textbf{Projection for training estimator}
% % Given the generated motion sequence data $\{\boldsymbol{\hat{X}}_{1:T}\}$, we project them to 2D to obtain paired training data.
% We consider two strategies for the projection: 
% 1) Heuristic random projection.
% % We set the virtual camera with certain elevation, azimuth range, height and distance range to match the {indoor capture environment}. This is similar to the projection strategy for 3D pose data synthesis as Chen~\et\cite{chen2016synthesizing};
% 2) Generative adversarial learning based projection~\cite{gong2021poseaug}. 
% % A generator is used to regress the camera orientation and position for each motion sequence. The regression is learned through a discriminator by distinguishing the real and the projected 2D pose sequences with the generated camera parameters.
% % In this way, reasonable camera viewpoint distribution can be extracted from real 2D pose data, improving the plausibility of generated 2D-3D paired data.
% % The two strategies are combined in our framework to ensure the diversity of camera viewpoints.

%%%%%%%%%%%%%%% detail of pose estimator - end %%%%%%%%%%%%%

\subsection{Pose imitator}
We here provide more detailed information on pose imitator $\mathcal{I}$.
As shown in Fig.~\ref{fig:imitator}, 
it contains reference motion, state, policy, action, and simulation environment.
Note that pose representation under 
imitation learning is based on joint axis angle $\boldsymbol{q}$,
which is convertible with joint position $\boldsymbol{X}$ through forward/inverse kinematics~\cite{mehta2017vnect}. 
Unless otherwise specified, 
the pose in this module is represented by 
joint axis angle $\boldsymbol{q}$ 
(\ie, reference motion $\boldsymbol{q}_{ref}$, velocity $\boldsymbol{q}'$, \etc).

\noindent \textbf{State} 
As shown in Fig.~\ref{fig:imitator},
the state includes current pose $\boldsymbol{q}_{t}$, current velocity $\dot{\boldsymbol{q}_{t}}$ from the simulation environment, 
target pose $\widetilde{\boldsymbol{q}}_{t+1}$ from reference motion, 
and an extra encoded feature $\phi$ encoded
by a temporal convolution network with a receptive field of 18,
which fuses the past and future reference motion information.
% To deal with the noisy reference motion from the pose estimator, we introduce an extra encoded feature $\phi$ by concatenating and fusing the past and future motion information.
% In this way, the control policy is aware of past and future reference motion, and is thus more robust to the noise.

\noindent \textbf{Action} involves two types of forces: internal force $\boldsymbol{\tau}_{t}$ and external force $\boldsymbol{\eta}_{t}$ as shown in Fig.~\ref{fig:imitator}. 
The internal force is applied by actuator on the non-root joints (\eg, elbow, knee). Following previous work~\cite{peng2017learning, yuan2020residual, yuan2021simpoe}, we use PD (proportional–derivative) control for internal force control.
% Moreover, residual strategy~\cite{yuan2021simpoe} is applied to further simplify the learning process. 
The internal force is formulated as:
\begin{equation}
\boldsymbol{\tau}_{t} = \boldsymbol{k}_p  (\boldsymbol{u}^{nr}_{t} - \boldsymbol{q}^{nr}_{t}) - \boldsymbol{k}_{d}  \dot{\boldsymbol{q}^{nr}_{t}}, \label{eq:trajloss}
\end{equation}
Where $\boldsymbol{k}_p, \boldsymbol{k}_{d}$ are the PD control parameters,
% $\boldsymbol{u}^{nr}_{t}$ is the residual angle for target PD pose $ \widetilde{\boldsymbol{q}}_{t+1} + \boldsymbol{u}^{nr}_{t}$, 
$\boldsymbol{u}^{nr}_{t}$ is the target angle for PD controller,
$\boldsymbol{q}^{nr}_{t}, \dot{\boldsymbol{q}^{nr}_{t}}$
is current joint pose and joint velocity, 
$\star^{nr}$ denotes non-root joint for non-root force $\boldsymbol{\tau}_{t}$ computation. 
The internal force $\boldsymbol{\tau}_{t}$, adjusted through the PD control parameters $\boldsymbol{k}_p, \boldsymbol{k}_{d}$ and target angle $\boldsymbol{u}^{nr}_{t}$ regressed by the policy network, drives the agent to target joint pose $\widetilde{\boldsymbol{q}}_{t+1}$ in desired time.
The external force $\boldsymbol{\eta}_{t}$ is a virtual 
force applied on root joint~(\ie, hip)~\cite{yuan2020residual} for
extra interaction (\eg, sitting on the chair) and is regressed by the policy network.
% \textcolor{red}{Consider that there are scenarios that require external object interaction such as sitting on the chairs, the external force is necessary to perform as a virtual chair to conduct such action. }
% Meanwhile, experiment in ~\cite{yuan2020residual} shows this force can further improve the training speed.
% With the PD control, residual angle, and external residual force, this pose imitator is able to handle varies of motion, and optimize in a faster speed compared with other approaches (\eg, DeepMimic~\cite{peng2018deepmimic} takes days to reproduce one motion clip). Besides it, the control policy only requires to train from scratch in the first cycle of our framework \nameofmethod{}. In the later cycle, the learned policy can be used as pretrained weight, easily adapted to the new incoming guidance signal.

%%%%%%%%%%%%%%%%%%%%%%
\begin{figure}[!t]
\centering
\includegraphics[width=0.95\linewidth]{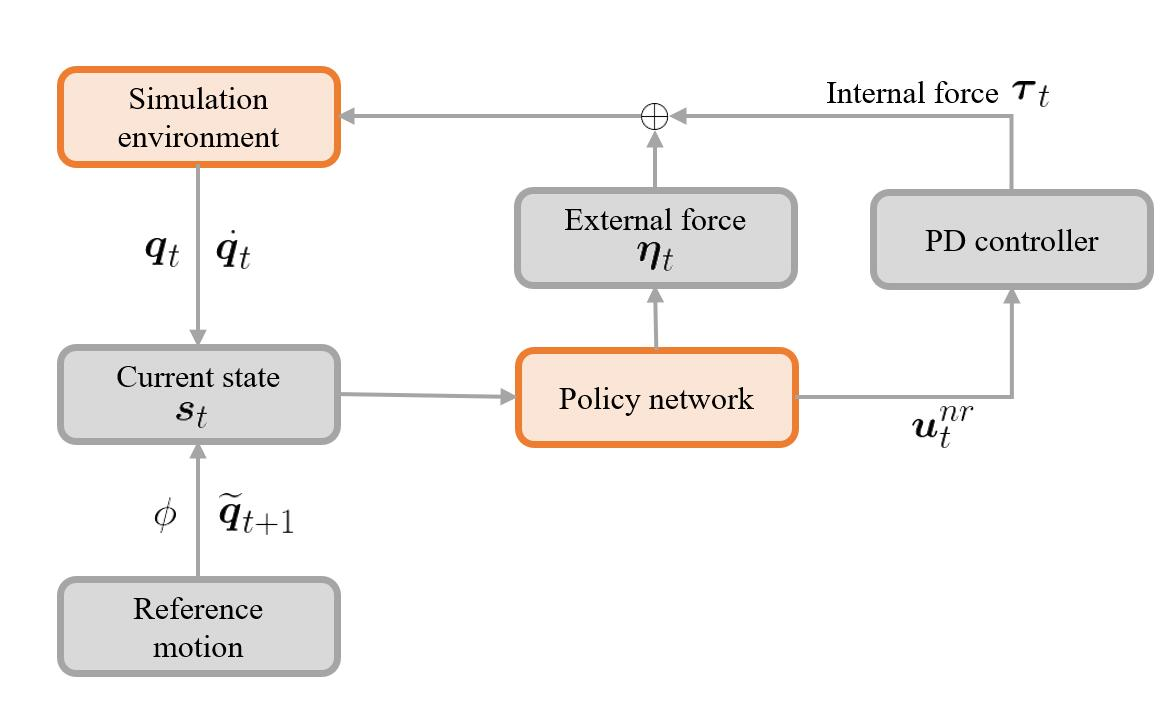}
\caption{\textbf{Pose imitator overview.}}
\label{fig:imitator}
\end{figure}
%%%%%%%%%%%%%%%%%%%%%%

\noindent \textbf{Rewards} 
measure the motion differences between the agent and reference motion. 
% matching certain characteristics of the reference motion
Following the  work~\cite{peng2018deepmimic, yuan2020residual}, 
the reward $\boldsymbol{r}_{t}$ here is formulated as:
%%%%%%%%%
\begin{equation}
    \begin{split}
    &\boldsymbol{r}_{t} = \sum_{i=1}^{n} \boldsymbol{w}^{i} e^{-\boldsymbol{k}_i \|\varphi^i_t \otimes \widetilde{\varphi}^i_t\|},  \\
    % \mathrm{where} \ \
    % &where \ \boldsymbol{r}^i_{t} = e^{-\boldsymbol{k}_i \|\varphi^i_t \otimes \widetilde{\varphi}^i_t\|}, \label{eq:reward}
    \end{split}    
\end{equation}
% \vspace{-0.75mm}
%%%%%%%%%%%%%%%%%%%%%%%%%%%%%
% where $\boldsymbol{r}_{t}$ is the rewards at time $t$, $\boldsymbol{r}^i_{t}$ is the sub rewards for different motion characteristics $\varphi^i_t$, $\boldsymbol{w}^{i}$ is the corresponding weight factor.
where $\boldsymbol{w}^{i}, \boldsymbol{k}_i, \varphi^i_t, \widetilde{\varphi}^i_t$ 
are the weight factor, scale factor, motion characteristics, 
% (\ie, pose $\boldsymbol{q}_{t}$, velocity $\dot{\boldsymbol{q}_{t}}$, \etc), 
and reference motion characteristics, respectively.
The operation $\otimes$ compute the distance between the agent 
motion property $\varphi^i_t$ and reference motion property $\widetilde{\varphi}^i_t$.
Such differences capture pose related (pose, velocity), root related (root height, root velocity) and body-end factors (position, velocity in end-effector \ie, feet, hand and head).
Besides, a regulation loss on virtual force is applied to 
avoid unnecessary external force~\cite{yuan2020residual}, which is formatted as:
%%%%%%%%%
\begin{equation}
    \begin{split}
    % &\boldsymbol{r}_{t} = \sum_{i=1}^{n} \boldsymbol{w}^{i} e^{-\boldsymbol{k}_i \|\varphi^i_t \otimes \widetilde{\varphi}^i_t\|},  \\
    % % \mathrm{where} \ \
    \boldsymbol{r}^{\boldsymbol{\eta}_{}}_{t} = e^{-\boldsymbol{k}_{\boldsymbol{\eta}_{}} \|\boldsymbol{\eta}_{t}\|}, \label{eq:reward}
    \end{split}    
\end{equation}
% \vspace{-0.75mm}$\boldsymbol{\eta}_{t}$
%%%%%%%%%%%%%%%%%%%%%%%%%%%%%
where $\boldsymbol{r}^{\boldsymbol{\eta}_{}}_{t}, \boldsymbol{k}_{\boldsymbol{\eta}_{}}, \boldsymbol{\eta}_{t}$ 
are the virtual force rewards, scale factor, virtual force, respectively. 
As we find that 
it is hard for the agent to 
move with the above setting 
due to the noisy reference motion, 
we further introduce a feet relative 
position (\ie, a vector from left foot point to right foot)
into the motion characteristics
% which measures the vector from one foot to another 
to enhance the feet motion.
Note that all these motion characteristics 
are measured in local heading coordinate
system, following previous works~\cite{yuan2019ego, yuan2020residual}. 
%This is to avoid large error accumulation compared with world coordinate system.

% The different motion characteristics $\varphi^i_t$ include joint angle, joint angle velocity, end effector position, root height, root linear velocity, root angler velocity, foot relative vector.
% In sub rewards computation, $\otimes$ calculates the distance between the agent motion property $\varphi^i_t$ and reference motion property $\widetilde{\varphi}^i_t$ (\ie, L2 distance for scalar property such as linear velocity, height. quaternion distance for angler property such as joint pose, joint pose velocity). $\boldsymbol{k}_i$ is scale factor to ensure the exponential power factor in suitable range (\ie, we set all initial power factor for the exponential value of 0.5) for proper rewards gradient.

% % put in supplementary
\noindent \textbf{Initial Condition} 
For the {initial condition}, instead of using the starting pose~\cite{yuan2019ego, yuan2020residual}, 
we set the initial pose as T pose.
Since the pose signal in our \nameofmethod{} contains
more noises compared to  conventional RL tasks,
it may yield the initialization crash;
such an initial condition, in practice,
helps us to avoid simulation 
crush.

\noindent \textbf{Termination Condition} 
% We terminate the algorithm
For the {termination condition}, we set it as when head height is 0.3~m below the reference head height or episode (\ie, reference motion) end.

\subsection{Pose hallucinator}
% The pose hallucinator aims to generate novel and diverse motion sequence based on the refined data from pose imitator. 
% There are various methods that can generate novel motion, including motion prediction~\cite{yuan2020dlow, pavllo2018quaternet} and motion interpolation~\cite{kaufmann2020convolutional, duan2021ssmc, harvey2020robust}.
% In this work, we choose motion interpolation technique to generate novel pose motions. Specifically, we sample key-frames from the refined pose sequence, and interpolate the missing frames via neural networks to generate new motion data.
% In details, the pose hallucinator is constructed by a recurrent neural network (RNN) structure. The inputs are the sampled temporal key-frames (we sample key-frames with a certain frame interval).
% Conditioned on these sampled key-frames, the model predicts the intermediate frames in sequential manner.
% A reconstruction loss and an adversary loss is used to train this model.
% The reconstruction loss measures the $L_2$ distance between the ground truth and predicted poses. The adversary loss provides temporal supervision to avoid RNN collapse (\ie, predicting average motion).
% In the inference stage, we randomly select frames from different motion clips and generate novel motion sequences based on these sampled key-frames.

%%%%%%%%%%%%%%%%%%%%%%
\begin{figure}[!t]
\centering
\includegraphics[width=0.85\linewidth]{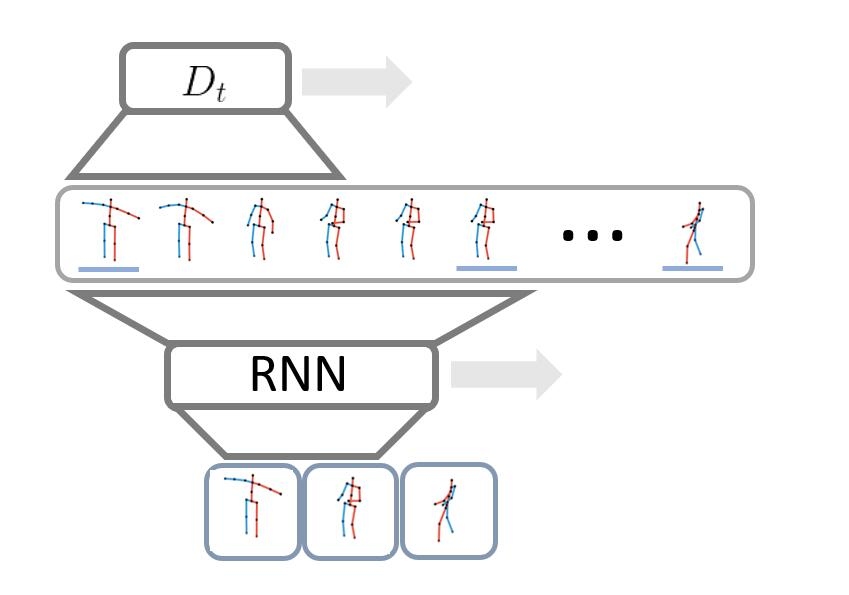}
\caption{\textbf{Pose hallucinator overview.}}
\label{fig:hallucinator}
\end{figure}
%%%%%%%%%%%%%%%%%%%%%%
{For the pose hallucinator, we adopt the motion interpolation based approach~\cite{harvey2020robust} as it can generate arbitrary length sequence with continuously input key frames.
Fig~\ref{fig:hallucinator} illustrates the architecture of
pose hallucinator. 
It contains a conditional RNN generator, and a temporal discriminator. 
During training stage, The RNN generator, condition on the sampled key frames, recover the masked intermediate frames.
The temporal discriminator sliding on the recovered pose sequence, provides guidance to encourage the temporal motion plausibility. 
Another reconstruction loss is applied to measure the difference between recovered pose sequence and original one.
During the inference stage, random sampled key frames are used as input, and generate unseen motion though the conditional RNN generator, which is then used as diversified reference motion for the imitator.  
}

\section{Negative social impact} 
Our method can be applied to lots of 3D
pose estimation related applications including action recognition and human
tracking, etc, but may involves user privacy issues.
